# Supplementary material for: Neural Sinkhorn Gradient Flow
Source: arXiv:2401.14069 source file (2024-01-25)
Supplement: Supplementary file 1 [file Algroithm_add.tex]

\section{Inference Algorithm}\label{Inference algorithm}
\begin{algorithm}
    \resizebox{0.47\textwidth}{!}{\begin{minipage}{\linewidth}
    % \SetKwFunction{isOddNumber}{isOddNumber}
    % \SetAlgoNlRelativeSize{0.5}
    \SetKwInOut{KwIn}{Input}
    \SetKwInOut{KwOut}{Output}
 
    \KwIn{number of time steps $T$, inference step size $\eta$, time-varying velocity field $\vv^\theta$, prior samples $ \tilde{X}_i^0 \sim \tilde{\mu}_0$}
    
    \For{$t = 0, 1, \cdots T$}{
       $\tilde{X}_i^{t+1}=\tilde{X}_i^t+\eta \vv^\theta\left(\tilde{X}_i^t, t\right), i=1,2, \cdots n . $ 
    }
    
    \KwOut{$\tilde{X}_i^{T}$ as the results.}
 
 \caption{\textbf{Inference via velocity field} }
 \label{velocity field inference}
 \end{minipage}
 }
 \end{algorithm}
